# Supplementary material for: Interact with me: Joint Egocentric Forecasting of Intent to Interact, Attitude and Social Actions
Source: arXiv:2412.16698 source file (2025-05-08)
Supplement: Supplementary file 2 [file main.tex]

\section*{Appendix}

\subsection{Comparison between JPL and JPL-Social}

The JPL \cite{JPL, jplextension} dataset concerns only about the action that the interacting subjects are performing. By comparison, our JPL-Social dataset also provides annotations of each person's intent to interact and attitude of interaction. Another difference is that the JPL \cite{JPL, jplextension} dataset only provides video-level labels, i.e., each video clip is labeled with the action of those interacting subjects who are also at the center of the field of view. By comparison, our dataset JPL-Social, offers labels of each person in the view.
